# Supplementary material for: Data-Driven Physical Face Inversion
Source: arXiv:1907.10402 source file (2019-07-24)
Supplement: Supplementary file 1 [file appendix.tex]

\section{Appendix}\label{sec:appendix}

For $\mathbf{A}$ invertible square matrix, and $\mathbf{B}$ square matrix

\begin{align}
\mathbf{A X} & = \mathbf {B} \\
\mathbf{X}   & = \mathbf{A^{-1} B} \\
\mathbf{v}^\intercal \mathbf {X} & = \mathbf{ v^\intercal A^{-1} B} \\
\mathbf{v^\intercal X} & = \mathbf{y^\intercal B} \\
\end{align}

This means that in order to compute the term $\mathbf v^{\intercal}X$ it is sufficient to solve the system: $\mathbf{A y = v}$ 

In our case:

$\mathbf A = \frac{\partial^2 E_{\text{int}}(\mathbf{X}, \mathbf{x})}{\partial \mathbf{x}^2} $

$\mathbf B = -\frac{\partial^2 E_{\text{int}}(\mathbf{X}, \mathbf{x})}{\partial \mathbf{X} \partial \mathbf{x}} + \frac{\partial \mathbf{f}_{\text{ext}}(\mathbf{X})}{\partial \mathbf{X}}$

$v = \left( \mathbf{x}_j - \bar{\mathbf{x}}_j \right) $

$\mathbf{X} =  \frac{\partial \mathbf{x}_j(\mathbf{X})}{\partial \mathbf{X}}$

Leading to the equation system:
\begin{equation}
\frac{\partial^2 E_{\text{int}}(\mathbf{X}, \mathbf{x})}{\partial \mathbf{x}^2} \; \mathbf{y} = \left( \mathbf{x}_j - \bar{\mathbf{x}}_j \right)
\end{equation}
